# Supplementary material for: Disentangling Quantum and Classical Contributions in Hybrid Quantum Machine Learning Architectures
Source: arXiv:2311.05559 source file (2024-01-13)
Supplement: Supplementary file 1 [file X_appendix.tex]

%\section*{\uppercase{Appendix}}
